# Supplementary material for: Network Momentum across Asset Classes
Source: arXiv:2308.11294 source file (2023-08-22)
Supplement: Supplementary file 1 [file appendix-dataset1-commod.tex]

\clearpage

\begin{table}[h!]
\centering
\small
\caption{The Pinnacle Universe}
\label{table:universe}
\begin{tabular}{lll}
\toprule
\textbf{\centering Ticker} & \textbf{\centering Description } & \textbf{\centering Period}\\
\midrule
\textbf{Commodities:} \\
BC & BRENT CRUDE OIL, composite & 2010-2022 \\
BG & BRENT GASOIL, composite & 2010-2022 \\
CC & COCOA & 1990-2022 \\
CL & CRUDE OIL & 1990-2021 \\
CT & COTTON \#2 & 1990-2022 \\
DA & MILK III, composite & 1999-2022 \\
GI & GOLDMAN SAKS C. I. & 1995-2022 \\
JO & ORANGE JUICE & 1990-2022 \\
KC & COFFEE & 1990-2022 \\
KW & WHEAT & 1990-2022 \\
LB & LUMBER & 1990-2022 \\
MW & WHEAT, MINN & 1990-2022\\
NR & NATURAL GAS & 1990-2021 \\
SB & SUGAR \#11 & 1990-2022 \\
W\_ & WHEAT, CBOT & 1990-2018 \\
ZA & PALLADIUM, electronic &1990-2022  \\
ZB & RBOB, electronic & 1990-2022 \\
ZC & CORN, electronic & 1990-2022\\
ZF & FEEDER CATTLE, electronic & 1990-2022 \\
ZG & GOLD, electronic & 1990-2022 \\
ZI & SILVER, electronic &1990-2022 \\
ZK & COPPER, electronic & 1990-2022\\
ZL & SOYBEAN OIL, electronic &1990-2022 \\
ZM & SOYBEAN MEAL, electronic &1990-2022 \\
ZN & NATURAL GAS, electronic & 1992-2022\\
ZO & OATS, electronic &1990-2022 \\
ZP & PLATINUM, electronic & 1990-2022\\
ZR & ROUGH RICE, electronic & 1990-2022 \\
ZS & SOYBEANS electronic & 1990-2022 \\
ZT & LIVE CATTLE, electronic & 1990-2022  \\
ZU & CRUDE OIL, electronic & 1990-2022\\
ZW & WHEAT electronic & 1990-2022 \\
ZZ & LEAN HOGS, electronic & 1990-2022 \\

\midrule
\textbf{Equities:} && \\
AX & GERMAN DAX INDEX & 1999-2022 \\
CA & CAC40 INDEX & 2000-2022 \\
EN & NASDAQ, MINI & 2001-2022 \\
ER & RUSSELL 2000, MINI & 2004-2022\\
ES & S\&P 500, MINI & 1999-2022 \\
HS & HANG SENG INDEX & 1999-2022 \\
LX & FTSE 100 INDEX & 1991-2022\\
MD & S\&P 400, MINI, electronic & 1994-2022 \\
SC & S\&P 500, composite & 1996-2022 \\
SP & S\&P 500, day session & 1990-2022 \\
XU & DOW JONES EUROSTOXX 50 & 2003-2022 \\
XX & DOW JONES STOXX 50 & 2004-2022 \\
YM & DOW JONES, MINI (\$5.00) & 2004-2022 \\

\midrule
\textbf{Fixed Income:} \\
AP &  AUSTRALIAN PRICE INDEX & 2010-2022 \\
DT &  EURO BOND (BUND) & 1991-2022\\
FB &  T-NOTE, 5yr composite &1990-2022\\
GS &  GILT, LONG BOND & 1991-2022\\
TU &  T-NOTES, 2yr composite & 1992-2022\\
TY &  T-NOTE, 10yr composite & 1990-2022\\
UB &  EURO BOBL & 2000-2022\\
US &  T-BONDS, composite & 1990-2022 \\

\midrule
\textbf{Currencies:} \\
AN & AUSTRALIAN \$\$, day session & 1990-2022 \\
BN & BRITISH POUND, composite & 1990-2022\\
CB & CANADIAN 10YR BOND & 1996-2022\\
CN & CANADIAN \$\$, composite & 1990-2022\\
DX & US DOLLAR INDEX & 1990-2022\\
FN & EURO, composite &1990-2022\\
JN & JAPANESE YEN, composite & 1990-2022\\
MP & MEXICAN PESO & 1997-2022\\
NK & NIKKEI INDEX & 1992-2022\\
SN & SWISS FRANC, composite &1990-2022 \\
\bottomrule
\end{tabular}
\end{table}
